# Supplementary material for: Thwarting Piracy: Anti-debugging Using GPU-assisted Self-healing Codes
Source: arXiv:2210.11047 source file (2022-10-20)
Supplement: Supplementary file 1 [file Appendix.tex]

\begin{lstlisting}[frame=single]
std::array<std::uint_fast32_t, 256>
    generate_crc_lookup_table() noexcept
{
    auto const reversed_polynomial = 
        std::uint_fast32_t{0xEDB88320uL};
    struct byte_checksum
    {
        std::uint_fast32_t operator()()
                            noexcept
        {
            auto checksum = static_cast
                <std::uint_fast32_t>(n++);
            for (auto i = 0; i < 8; ++i)
                checksum = 
                (checksum >> 1) ^ 
                ((checksum & 0x1u) ? 
                reversed_polynomial : 0);
            return checksum;
        }
        unsigned n = 0;
    };
    auto table = 
        std::array<std::uint_fast32_t,
            256>{};
    std::generate(table.begin(), 
                  table.end(), 
                  byte_checksum{});
    return table;
}

template <typename InputIterator>
std::uint_fast32_t 
crc(InputIterator first, 
    InputIterator last)
{
static auto const table = 
    generate_crc_lookup_table();
return std::uint_fast32_t{0xFFFFFFFFuL} &
    ~std::accumulate(first, last,
        ~std::uint_fast32_t{0} & 
        std::uint_fast32_t{0xFFFFFFFFuL},
        [](std::uint_fast32_t checksum, 
            std::uint_fast8_t value)
        { 
            return table[
                (checksum ^ value) & 
                0xFFu] ^ (checksum >> 8);
        });
}

bool isFunctionPatched(
    const unsigned char *func, 
    const size_t& machine_code_size, 
    const std::uint32_t& checksum)
{
    bool result = true;
    std::vector<unsigned char> 
        machine_code;
    for (auto i = 0; 
            i < machine_code_size; 
            ++i)
    {
        machine_code.push_back(*(func+i));
    }
    uint32_t value = 
        crc(machine_code.begin(), 
            machine_code.end());
    result = (value != checksum);
    return result;
}
\end{lstlisting}

\subsection{Reference implmentation for hardware breakpoint}
A reference implementation for break-point detection using \texttt{GetThreadContext} API is as below:

\begin{lstlisting} [frame=single]
bool isHardwareBreakpointPresent(
    const unsigned char *address, 
    const std::vector<unsigned int>& offsets)
{
    CONTEXT ctx;
    ZeroMemory(&ctx, sizeof(CONTEXT)); 
    
    ctx.ContextFlags = CONTEXT_DEBUG_REGISTERS; 
    HANDLE hThread = GetCurrentThread();

    if(GetThreadContext(hThread, &ctx) == 0)
        return -1;

    bool result = false;
    for (auto &i : offsets)
    {
        if (address + i == (unsigned char*)ctx.Dr0)
        {
            result = true;
            break;
        }
        if (address + i == (unsigned char*)ctx.Dr1)
        {
            result = true;
            break;
        }
        if (address + i == (unsigned char*)ctx.Dr2)
        {
            result = true;
            break;
        }
        if (address + i == (unsigned char*)ctx.Dr3)
        {
            result = true;
            break;
        }
    }
    
    return result;
}
\end{lstlisting}

\subsection{Reference implmentation for hardware breakpoint using ptrace}
A reference implementation for break-point detection using \texttt{ptrace} system is given below:

\begin{lstlisting} [frame=single]
#define DR_OFFSET(x) (user->u_debugreg + x)

unsigned long long getDebugRegister(
    const user* user, 
    const pid_t pid, 
    unsigned char index)
{
    unsigned long long result = 0;
    result = ptrace(PTRACE_PEEKUSER, pid, user->u_debugreg[index], 0);
    return result;
}

bool isHardwareBreakpointPresent(
    const user* user, 
    const pid_t pid, 
    const unsigned char *address, 
    const std::vector<unsigned int>& offsets)
{
    unsigned long long dr[4];
    
    for (int i = 0; i < 4; ++i)
    {
        dr[i] = getDebugRegister(user, pid, i);
    }
    
    bool result = false;
    for (auto& offset : offsets)
    {
        for (int i = 0; i < 4; ++i)
        {
            if (address + offset == (unsigned char*)dr[i])
            {
                result = true;
                break;
            }
        }
    }
    
    return result;
}
\end{lstlisting}

\subsection{Evade software break-point}
\begin{lstlisting} [frame=single]
#include <iostream>
#include <sys/mman.h>
#include <unistd.h>
#include <vector>

bool removeBreakpoint(
    unsigned char* func, 
    const std::vector<unsigned int>& offsets,
    const std::vector<unsigned char>& original_bytes)
{
    bool result = false;
    if (offsets.size() > original_bytes.size())
        return false;
        
    long pagesize = 
        sysconf(_SC_PAGESIZE);
    unsigned long page_start = 
        (unsigned long)func & 
        ~(pagesize - 1);
        
    if (mprotect(
            (void*)page_start, 
            pagesize, 
            PROT_READ | PROT_WRITE | PROT_EXEC) != 0)
    {
        std::cerr << "mprotect() failed" << std::endl;
        return false;
    }
    for (auto i = 0; i < offsets.size(); ++i)
    {
        if (*(func + offsets[i]) != original_bytes[i])
        {
            *(func + offsets[i]) = original_bytes[i];
            result = true;
        }
    }
    return result;
}

bool isBreakpointPresent(
    const unsigned char *func, 
    const std::vector<unsigned int>& offsets)
{
    bool result = false;
    for (auto &i : offsets)
    {
        if (*(func + i) == 0xCC)
        {
            result = true;
            break;
        }
    }
    return result;
}

void secret()
{
    for (int i = 0; i < 10; ++i)
    {
        std::cout << "Try a breakpoint at secret()" << std::endl;
    }
}

int main()
{
    auto *ptr_secret = (unsigned char*)secret;
    
    std::vector<unsigned int> offsets = 
        {0, 1, 4, 8, 15, 19, 21, 28, 
         35, 40, 43, 50, 53, 56, 61, 
         65, 67, 68, 69};
    
    std::vector<unsigned char> original_bytes = 
        {0x55, 0x48, 0x48, 0xc7, 0x83, 
         0x7f, 0x48, 0x48, 0xe8, 0x48, 
         0x48, 0x48, 0x48, 0xe8, 0x83, 
         0xeb, 0x90, 0xc9, 0xc3};
    
    if (isBreakpointPresent(ptr_secret, offsets)) 
    {
        std::cerr << "Breakpoint detected" << std::endl;
        if (removeBreakpoint(
                ptr_secret, 
                offsets, 
                original_bytes)) 
        {
            std::cout << "Breakpoint removed" << std::endl;
            secret();
        }
        else
            std::cerr << "Cannot remove breakpoint" << std::endl;
    }
    else
        secret();
    return 0;
}
\end{lstlisting}

This  code can be trivially enhanced to restore code in case of function patching, as shown below (code stripped to bare minimum):

\begin{lstlisting} [frame=single]
bool unpatchFunction(
    unsigned char *func, 
    const std::vector<unsigned char>& machine_code)
{
    bool result = false;

    long pagesize = sysconf(_SC_PAGESIZE);
    unsigned long page_start = 
        (unsigned long)func &
        ~(pagesize - 1);

    if (mprotect(
            (void*)page_start, 
            pagesize, 
            PROT_READ | PROT_WRITE | PROT_EXEC) != 0)
    {
        std::cerr << "mprotect() failed" << std::endl;
        return false;
    }

    for (auto i = 0; i < machine_code.size(); ++i)
    {
        if (*(func + i) != 
            machine_code[i]) 
            {
                *(func + i) = machine_code[i];
                result = true;
            }
    }

    return result;
}
\end{lstlisting}

\subsection{Memory break-point evasionr4}
A reference implementation for the above is given in appendix
\begin{lstlisting} [frame=single]
bool isMemoryBreakpointPresent()
{
unsigned char *pMem = NULL;
SYSTEM_INFO sysinfo = {0}; 
DWORD OldProtect = 0;
void *pAllocation = NULL;

GetSystemInfo(&sysinfo);

pAllocation = 
VirtualAlloc(
NULL, 
sysinfo.dwPageSize, 
MEM_COMMIT | MEM_RESERVE, 
PAGE_EXECUTE_READWRITE); 

if (pAllocation == NULL)
return false; 

pMem = (unsigned char*)pAllocation;
*pMem = 0xc3; 

if (VirtualProtect(
pAllocation, 
sysinfo.dwPageSize, 
PAGE_EXECUTE_READWRITE | PAGE_GUARD, 
&OldProtect) == 0)
{
return false;
} 

__try
{
__asm
{
mov eax, pAllocation
push MemBpBeingDebugged
jmp eax
}
}
__except(EXCEPTION_EXECUTE_HANDLER)
{
VirtualFree(
pAllocation, 
NULL, 
MEM_RELEASE);
return false;
}     

__asm{MemBpBeingDebugged:}
VirtualFree(
pAllocation, 
NULL, 
MEM_RELEASE);
return true;
}
\end{lstlisting}
